# Supplementary material for: Revealing the free energy landscape of halide perovskites: Metastability and transition characters in CsPbBr$_3$ and MAPbI$_3$
Source: arXiv:2307.12100 ancillary file (2023-10-07)
Supplement: Supplementary file 1 [file supporting-information.pdf]

## Supporting Information:

### Revealing the free energy landscape of halide perovskites: Metastability and transition characters in CsPbBr<sub>3</sub> and MAPbI<sub>3</sub>

Erik Fransson<sup>1</sup>, J. Magnus Rahm<sup>1</sup>, Julia Wiktor<sup>1</sup>, and Paul Erhart<sup>1,\*</sup>

<sup>1</sup> *Department of Physics, Chalmers University of Technology, SE-41296, Gothenburg, Sweden*  
*\*erhart@chalmers.se*

## Contents

|                                                           |           |
|-----------------------------------------------------------|-----------|
| <b>Supplemental Notes</b>                                 | <b>2</b>  |
| S1. Density functional theory calculations . . . . .      | 2         |
| S2. Quantifying the character of the transition . . . . . | 2         |
| <b>Supplemental Figures</b>                               | <b>3</b>  |
| <b>Supplemental Tables</b>                                | <b>10</b> |
| <b>Supplemental References</b>                            | <b>12</b> |

## Supplemental Notes

### Supplemental Note S1: Density functional theory calculations

Density functional theory (DFT) calculations were performed using the projector augmented-wave method<sup>1</sup> as implemented in the Vienna ab-initio simulation package.<sup>2,3</sup> To this end, the exchange-correlation contribution was represented using the strongly constrained and appropriately normed (SCAN) density functional.<sup>4</sup> The Brillouin zone was sampled with a  $\Gamma$ -centered grid with a  $\mathbf{k}$ -point density of  $0.25 \text{ \AA}^{-1}$  and Gaussian smearing with a width of 0.1 eV.

### Supplemental Note S2: Quantifying the character of the transition

To quantify the character of a transition, a double Gaussian can be fitted to the histogram  $p(x)$  of the energy and lattice parameters (Fig. S3 and Fig. S4)

$$p(x) = \frac{g}{\sigma_{\text{cub}}\sqrt{2\pi}} \exp\left[-\frac{(x - \mu_{\text{cub}})^2}{2\sigma_{\text{cub}}^2}\right] + \frac{1-g}{\sigma_{\text{tet}}\sqrt{2\pi}} \exp\left[-\frac{(x - \mu_{\text{tet}})^2}{2\sigma_{\text{tet}}^2}\right], \quad (\text{S1})$$

where  $\mu$  and  $\sigma$  are the mean and standard deviation of the normal distributions, and cub and tet refer to the cubic and tetragonal phase respectively. Here,  $g$  represents the relative occurrence of the cubic phase. The results of fitting the distributions to Eq. (S1) are shown by solid lines in Fig. S3 and Fig. S4.

## Supplemental Figures

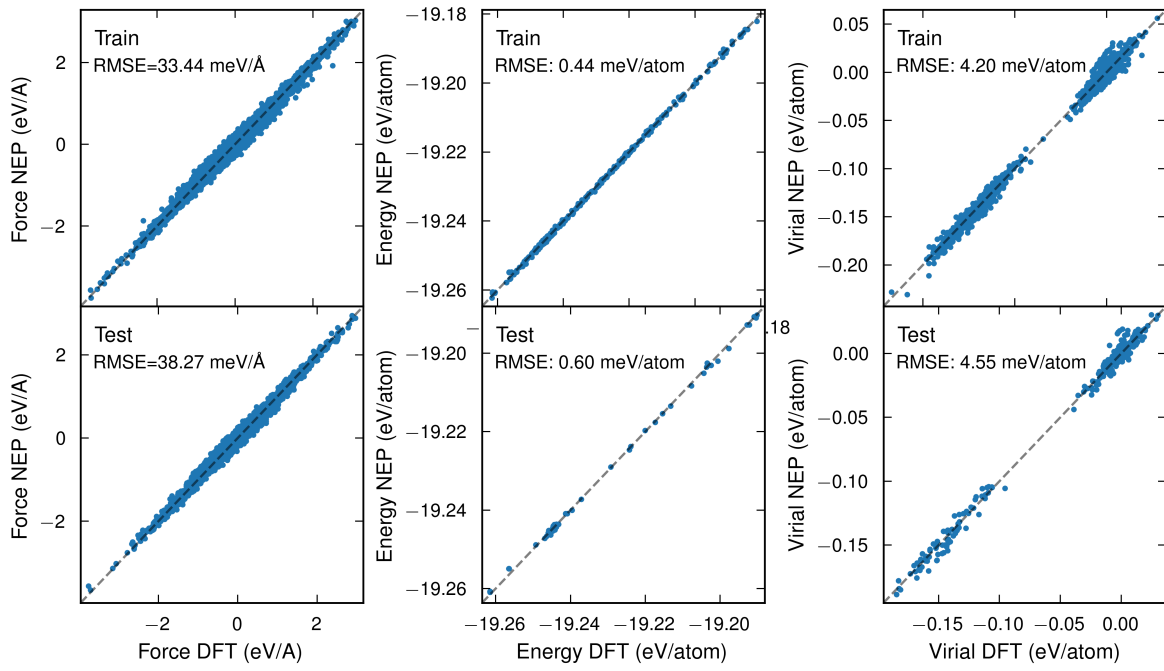

Figure S1: Parity plots for energies, forces, and virials for training (top) and test (bottom) data for the MAPI<sub>3</sub> model. A similar plot for the CsPbBr<sub>3</sub> model is available in<sup>5</sup>.

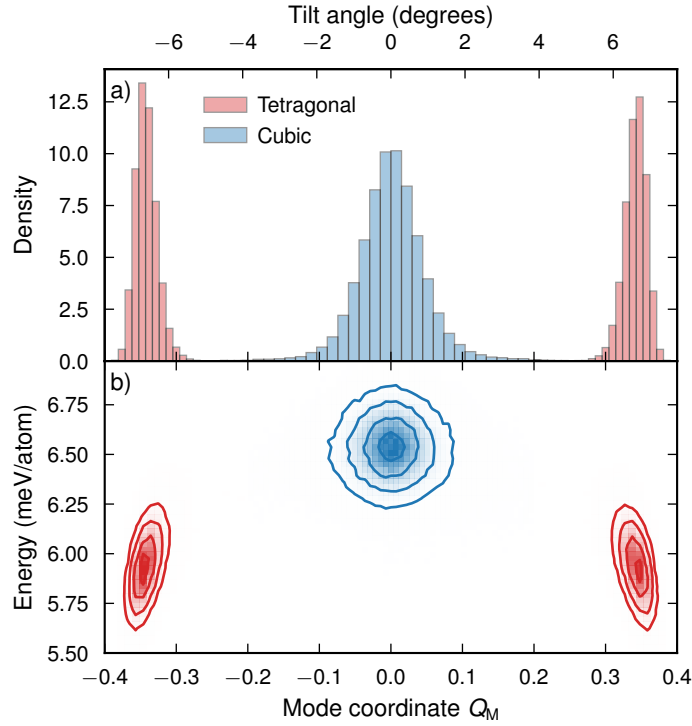

Figure S2: a) Distribution of the mode coordinate  $Q_M$  (corresponding tilt angles given in top x-axis) from large scale MD simulations at 302 K in the  $NpT$  ensemble for  $\text{CsPbBr}_3$ . The histograms are collected from the same set of MD simulations, and are colored depending if the mode coordinate is around zero (cubic) or not (tetragonal). From the mode histogram we can see that there is a region between the cubic and tetragonal which is almost never visited in the MD simulations indicating a barrier between the two phases. b) Joint distribution over the energy and the mode coordinate, clearly indicating that the tetragonal phase has a different energy then the cubic at this temperature.

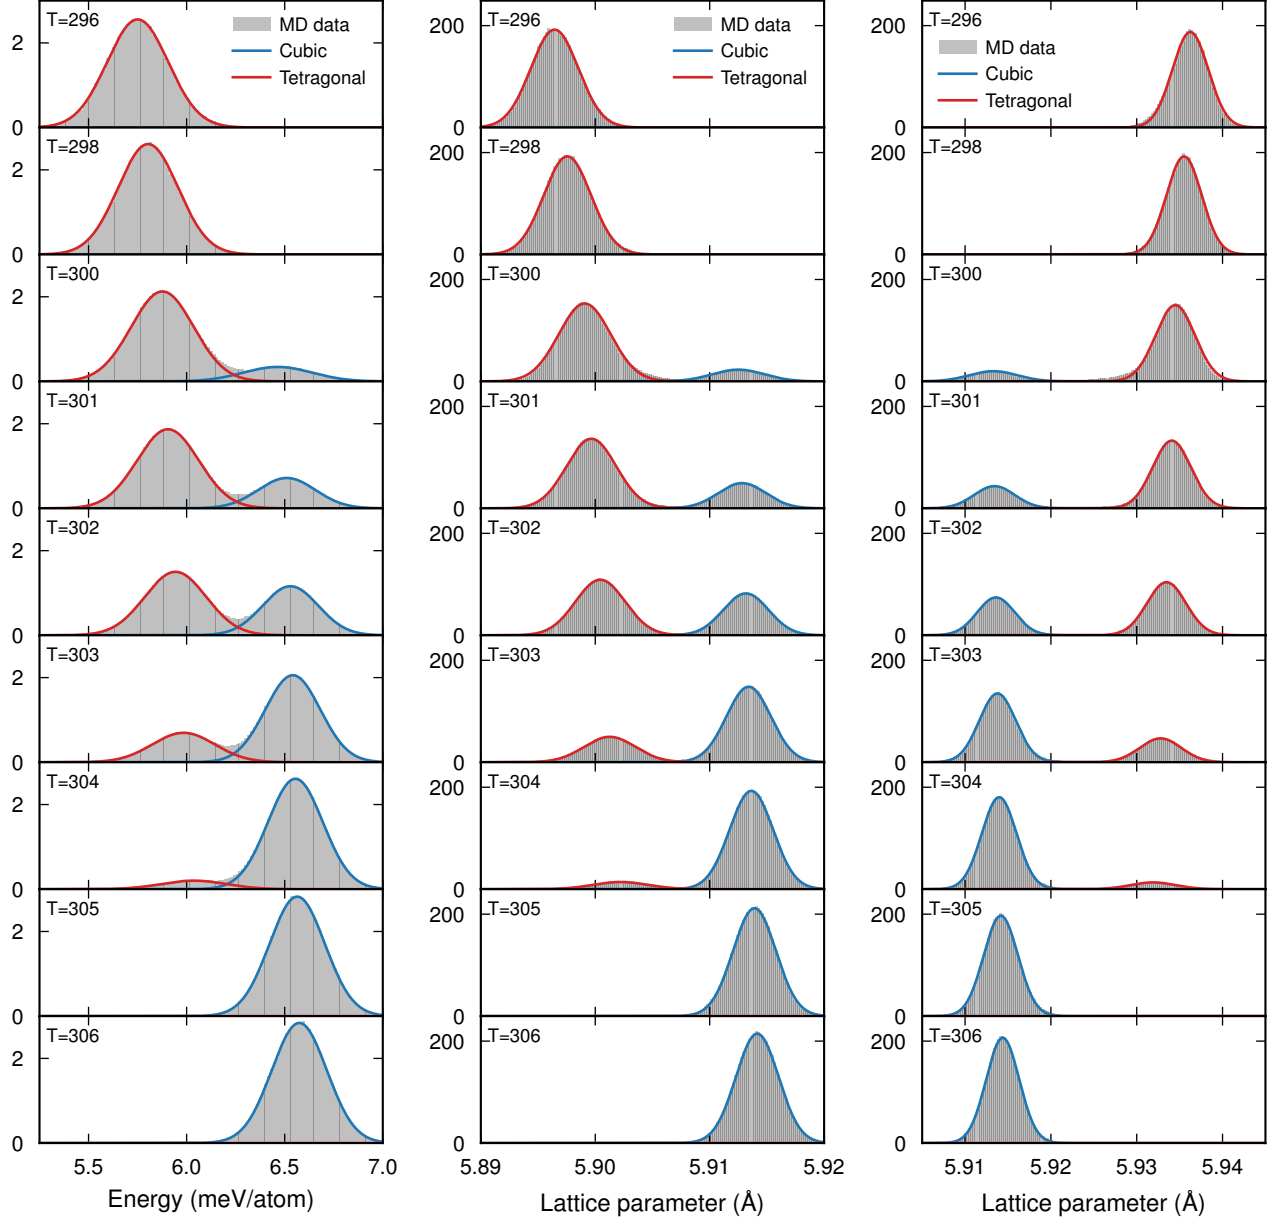

Figure S3: Distribution of the MD data and corresponding Gaussian fits, see Eq. (S1), for various temperatures for  $\text{CsPbBr}_3$ . The middle panel shows the lattice parameter  $a$ , and the rightmost column the lattice parameter  $c$ .

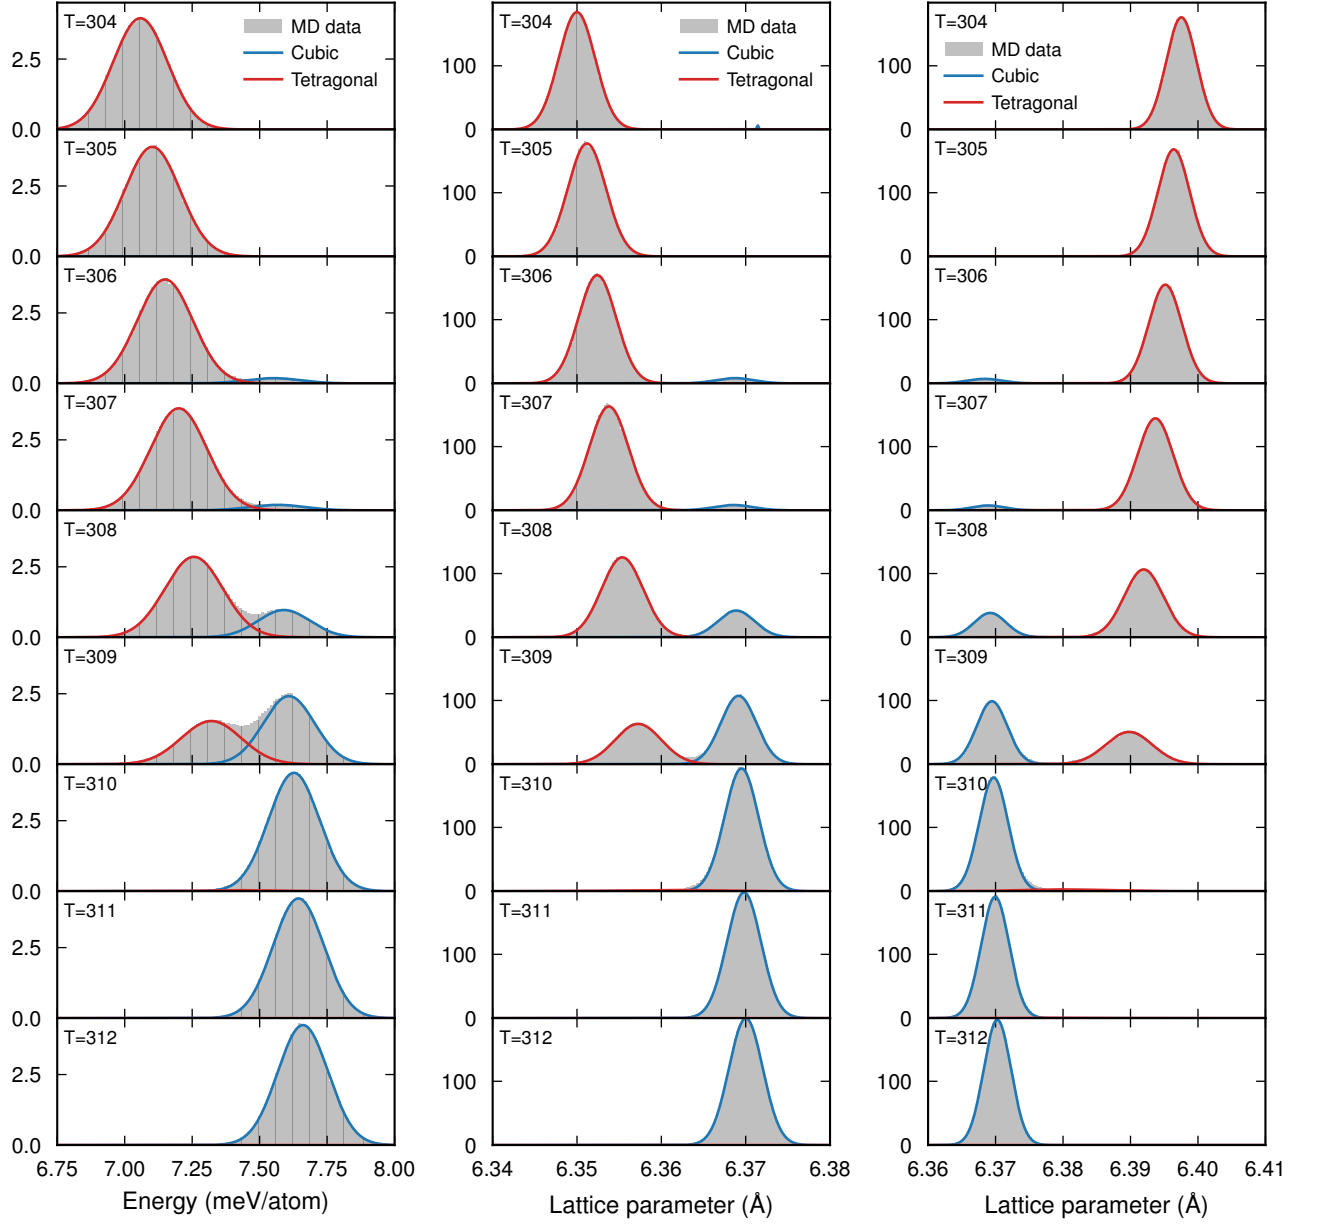

Figure S4: Distribution of the MD data and corresponding Gaussian fits, see Eq. (S1), for various temperatures for  $\text{MAPI}_3$ . The middle panel shows the lattice parameter  $a$ , and the rightmost column the lattice parameter  $c$ .

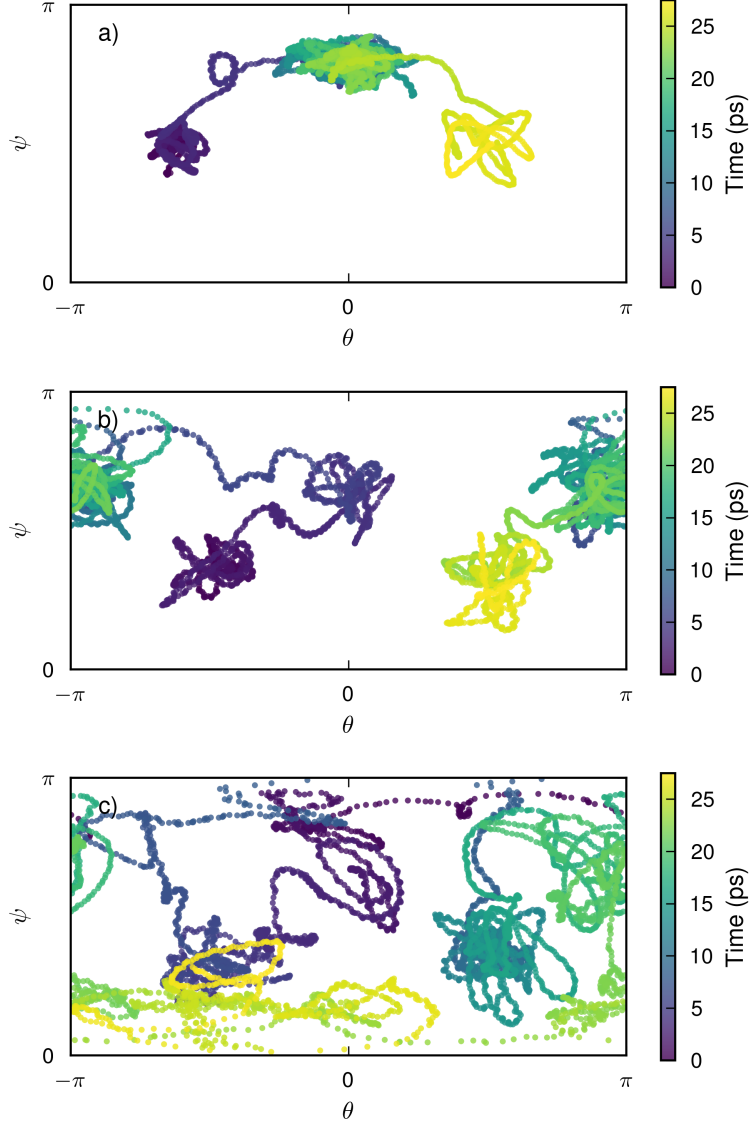

Figure S5: Time evolution of the orientation of a single C–N bond vector in a MA molecule from MD simulations for a) the  $a^-a^-c^+$  phase at 120 K, b) the  $a^0a^0c^-$  phase at 240 K, and c) the  $a^0a^0a^0$  at 340 K. Here,  $\theta$  refers to the angle in the x-y plane (azimuthal) and  $\phi$  to the angle to the z-axis (polar). The color indicates the simulation time. For the tetragonal and orthorhombic phases the  $c^-$  and  $c^+$  tilt axis is oriented along the z-axis.



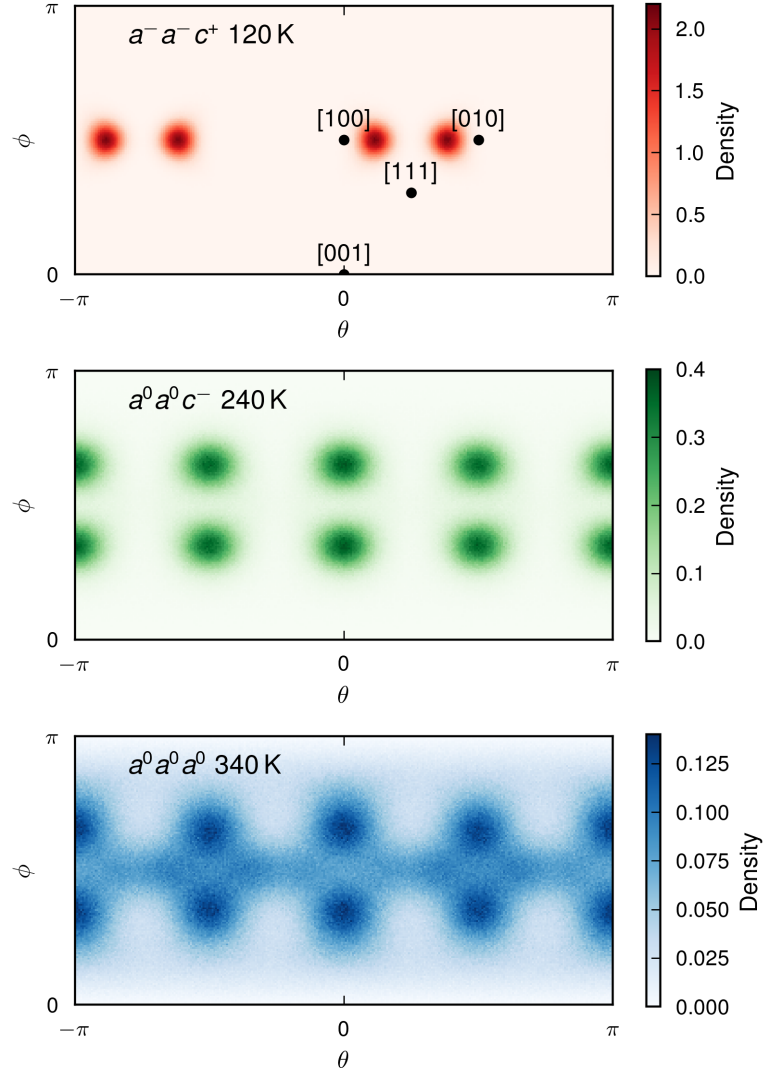

Figure S6: Distribution of the C-N vectors in the MA molecules from MD simulations. Here,  $\theta$  refers to angle in the x-y plane (azimuthal) and  $\phi$  to the angle to the z-axis (polar). For the tetragonal and orthorhombic phase the  $c^-$  and  $c^+$  tilting axis in the MD simulation is oriented along the z-axis.

## Supplemental Tables

Table S1: Energies obtained using DFT and NEP calculations for the lowest energy structure found for different MAPbI<sub>3</sub> phases.

| Structure   | DFT Energy (meV/f.u.) | NEP Energy (meV/f.u.) |
|-------------|-----------------------|-----------------------|
| $a^-a^-c^+$ | 0.0                   | 0.0                   |
| $a^0a^0c^-$ | 11.6                  | 19.6                  |
| $a^0a^0c^+$ | 33.4                  | 43.6                  |
| $a^0b^-b^-$ | 24.0                  | 35.7                  |

## Supplemental References

- [1] P. E. Blöchl. Projector augmented-wave method. *Physical Review B*, 50:17953, 1994. doi: 10.1103/PhysRevB.50.17953.
- [2] G. Kresse and J. Hafner. Ab initio molecular dynamics for liquid metals. *Physical Review B*, 47:558, 1993. doi: 10.1103/PhysRevB.47.558.
- [3] G. Kresse and J. Furthmüller. Efficiency of ab-initio total energy calculations for metals and semiconductors using a plane-wave basis set. *Computational Materials Science*, 6(1):15, 1996. doi: 10.1016/0927-0256(96)00008-0.
- [4] Jianwei Sun, Adrienn Ruzsinszky, and John P. Perdew. Strongly constrained and appropriately normed semilocal density functional. *Physical Review Letters*, 115:036402, 2015. doi: 10.1103/PhysRevLett.115.036402.
- [5] Erik Fransson, Petter Rosander, Fredrik Eriksson, J. Magnus Rahm, Terumasa Tadano, and Paul Erhart. Limits of the phonon quasi-particle picture at the cubic-to-tetragonal phase transition in halide perovskites. *Communications Physics*, 6(1), July 2023. doi: 10.1038/s42005-023-01297-8.
